# Supplementary material for: Wooly Graphs : A Mathematical Framework For Knitting
Source: arXiv:2407.00511 source file (2024-07-03)
Supplement: Supplementary file 1 [file Appendix.tex]

\begin{figure}[p]

\centering
\subfloat[Graph view with defined Hamiltonian path in red, note stitch 5 has only connections along the Hamiltonian path.  Stiches 2 and 8 have connections not shown that are not along the Hamiltonian path.]{\label{fig:basic_ham}
\centering
\resizebox{0.5\columnwidth}{!}{
\begin{tikzpicture}[->,>=stealth',shorten >=1pt,auto,node distance=2.1cm, semithick,black!30!blue]
    \tikzstyle{state} = [draw=none,fill=none,right]
    \tikzstyle{rec} = \tikzstyle{transition}=[rectangle,thick,draw=blue!75,minimum size=4mm]
    \tikzstyle{cir}=[ellipse,thick,draw=black!30!blue,minimum size=4mm, text=black!30!blue]
    \tikzstyle{di}=[diamond,thick,draw=blue!75,minimum size=4mm]

  \node[cir] (1)            {1};
  \node[cir] (2) [right =1.6cm of 1]                    {2};
  \node[cir] (3) [right  =1.6cm of 2]      {3};
  \node[cir] (4) [above =1.2cm of 3]                 {4};
  \node[cir] (5) [left =1.6cm of 4]                 {5};
  \node[cir] (6) [left =1.6cm of 5]      {6};
  \node[cir] (7)  [above =1.2cm of 6]          {7};
  \node[cir] (8) [right =1.6cm of 7]                    {8};
  \node[cir] (9) [right  =1.6cm of 8]      {9};
 \path (1) 
            edge[->,red] node {} (2)
            edge[-] node {} (6) 
        
        (2)
            edge[->,red] node {} (3)
        (3)
            edge[->,red] node {} (4)
        (4)
            edge[->,red] node {} (5)
        (5)
            edge[->,red] node {} (6)
        (6)
            edge[->, red] node {} (7)
        (7) 
            edge[->, red] node {} (8)
        (8)
            edge[->, red] node {} (9)
        (9)
            edge[-] node {} (4);
\end{tikzpicture}}
    }
%no space
\hfill
\subfloat[Knitting object created from the graph, note some basic stockinette is put around the graph-defined area for fabric stability.]{\label{fig:bo_example}
\centering

\includegraphics[width=0.45\linewidth]{images/knit_bo.jpeg}
}

\caption{This figure looks at nodes that have only connections along the Hamiltonian path.  For node 5, we cast on and immediately bind off to get the correct connections.}
\end{figure}

begin{figure}[p]

\centering
\subfloat[Graph view with defined Hamiltonian path in red.]{\label{fig:basic_ham}
\centering
\resizebox{0.5\columnwidth}{!}{
\begin{tikzpicture}[->,>=stealth',shorten >=1pt,auto,node distance=2.1cm, semithick,black!30!blue]
    \tikzstyle{state} = [draw=none,fill=none,right]
    \tikzstyle{rec} = \tikzstyle{transition}=[rectangle,thick,draw=blue!75,minimum size=4mm]
    \tikzstyle{cir}=[ellipse,thick,draw=black!30!blue,minimum size=4mm, text=black!30!blue]
    \tikzstyle{di}=[diamond,thick,draw=blue!75,minimum size=4mm]

  \node[cir] (1)            {1};
  \node[cir] (2) [right =1.6cm of 1]                    {2};
  \node[cir] (3) [right  =1.6cm of 2]      {3};
  \node[cir] (4) [above =1.2cm of 3]                 {4};
  \node[cir] (5) [left =1.6cm of 4]                 {5};
  \node[cir] (6) [left =1.6cm of 5]      {6};
 \path (1) 
            edge[->,red] node {} (2)
            edge[-] node {} (6) 
        
        (2)
            edge[->,red] node {} (3)
            edge[-] node {} (5)
        (3)
            edge[->,red] node {} (4)
        (4)
            edge[->,red] node {} (5)
        (5)
            edge[->,red] node {} (6);
\end{tikzpicture}}
    }
%no space
\hfill
\subfloat[Knitting object created from the graph, note some basic stockinette is put around the graph-defined area for fabric stability.]{\label{fig:ham_knit}
\centering

\includegraphics[width=0.45\linewidth]{images/1.png}
}

\subfloat[Graph view with defined Hamiltonian path in red.  Here we begin our path with node 2, which gives a different stitch pattern.]{\label{fig:ham_2}
\centering
\resizebox{0.5\columnwidth}{!}{
\begin{tikzpicture}[->,>=stealth',shorten >=1pt,auto,node distance=2.1cm, semithick,black!30!blue]
    \tikzstyle{state} = [draw=none,fill=none,right]
    \tikzstyle{rec} = \tikzstyle{transition}=[rectangle,thick,draw=blue!75,minimum size=4mm]
    \tikzstyle{cir}=[ellipse,thick,draw=black!30!blue,minimum size=4mm, text=black!30!blue]
    \tikzstyle{di}=[diamond,thick,draw=blue!75,minimum size=4mm]

  \node[cir] (1)            {2};
  \node[cir] (2) [right =1.6cm of 1]                    {3};
  \node[cir] (3) [right  =1.6cm of 2]      {4};
  \node[cir] (4) [above =1.2cm of 3]                 {5};
  \node[cir] (5) [left =1.6cm of 4]                 {6};
  \node[cir] (6) [left =1.6cm of 5]      {1};
 \path (1) 
            edge[->,red] node {} (2)
            edge[-] node {} (6) 
            edge[-] node {} (4)
        
        (2)
            edge[->,red] node {} (3)
        (3)
            edge[->,red] node {} (4)
        (4)
            edge[->,red] node {} (5)
        (5)
            edge[->,red] node {} (6);
\end{tikzpicture}}
    }
%no space
\hfill
\subfloat[Knitting object created from the graph, note some basic stockinette is put around the graph-defined area for fabric stability.]{\label{fig:ham_2_knit}
\centering

\includegraphics[width=0.45\linewidth]{images/4.png}
}

\subfloat[Graph view with defined Hamiltonian path in red.  Here we put the first four nodes on the first row, which gives a different knitted object.]{\label{fig:ham_3}
\centering
\resizebox{0.5\columnwidth}{!}{
\begin{tikzpicture}[->,>=stealth',shorten >=1pt,auto,node distance=2.1cm, semithick,black!30!blue]
    \tikzstyle{state} = [draw=none,fill=none,right]
    \tikzstyle{rec} = \tikzstyle{transition}=[rectangle,thick,draw=blue!75,minimum size=4mm]
    \tikzstyle{cir}=[ellipse,thick,draw=black!30!blue,minimum size=4mm, text=black!30!blue]
    \tikzstyle{di}=[diamond,thick,draw=blue!75,minimum size=4mm]

  \node[cir] (1)            {1};
  \node[cir] (2) [right =1.6cm of 1]                    {2};
  \node[cir] (3) [right  =1.6cm of 2]      {3};
  \node[cir] (4) [right =1.2cm of 3]                 {4};
  \node[cir] (5) [above =1.6cm of 4]                 {5};
  \node[cir] (6) [left =1.6cm of 5]      {6};
 \path (1) 
            edge[->,red] node {} (2)
            edge[-] node {} (6) 
        
        (2)
            edge[->,red] node {} (3)
            edge[-] node {} (5)
        (3)
            edge[->,red] node {} (4)
        (4)
            edge[->,red] node {} (5)
        (5)
            edge[->,red] node {} (6);
\end{tikzpicture}}
    }
%no space
\hfill
\subfloat[Knitting object created from the graph, note some basic stockinette is put around the graph-defined area for fabric stability.]{\label{fig:ham_3_knit}
\centering

\includegraphics[width=0.45\linewidth]{images/3.png}
}

\caption{An example of how different Hamiltonian paths can lead to different knitted objects.}
\label{fig:total_ham_path_fig}
\end{figure}

\begin{figure}[p]

\centering
\subfloat[Graph with defined Eulerian edges. We let red correspond to the edges being in back.  This corresponds to knit stitch or stockinette. ]{\label{fig:stockinette_graph}
\centering
\resizebox{0.5\columnwidth}{!}{
\begin{tikzpicture}[->,>=stealth',shorten >=1pt,auto,node distance=2.1cm, semithick,black]
    \tikzstyle{state} = [draw=none,fill=none,right]
    \tikzstyle{rec} = \tikzstyle{transition}=[rectangle,thick,draw=blue!75,minimum size=4mm]
    \tikzstyle{cir}=[ellipse,thick,draw=black,minimum size=4mm, text=black]
    \tikzstyle{di}=[diamond,thick,draw=blue!75,minimum size=4mm]

  \node[cir] (1)            {1};
  \node[cir] (2) [right =1.6cm of 1]                    {2};
  \node[cir] (3) [right  =1.6cm of 2]      {3};
  \node[cir] (4) [above =1.2cm of 3]                 {4};
  \node[cir] (5) [left =1.6cm of 4]                 {5};
  \node[cir] (6) [left =1.6cm of 5]      {6};
 \path (1) 
            edge[->] node {} (2)
            edge[->,red, bend left] node {} (6) 
        
        (2)
            edge[->] node {} (3)
            edge[->, red, bend left] node {} (5)
        (3)
            edge[->] node {} (4)
            edge[->, red, bend left] (4)
        (4)
            edge[->] node {} (5)
            edge[->,red, bend left] (3)
        (5)
            edge[->] node {} (6)
            edge[->,red,bend left] node {} (2)
        (6)
            edge[->,red,bend left] node {} (1);
\end{tikzpicture}}
    }
%no space
\hfill
\subfloat[Stockinette stitch, corresponding to the Eulerian edges being in back.]{\label{fig:stockinette}
\centering

\includegraphics[width=0.45\linewidth]{images/1.png}
}

\subfloat[Graph with defined Eulerian edges. We let blue mean the edges are in front.  This corresponds to purl stitch or reverse stockinette. ]{\label{fig:reverse_stockinette_graph}
\centering
\resizebox{0.5\columnwidth}{!}{
\begin{tikzpicture}[->,>=stealth',shorten >=1pt,auto,node distance=2.1cm, semithick,black]
    \tikzstyle{state} = [draw=none,fill=none,right]
    \tikzstyle{rec} = \tikzstyle{transition}=[rectangle,thick,draw=blue!75,minimum size=4mm]
    \tikzstyle{cir}=[ellipse,thick,draw=black,minimum size=4mm, text=black]
    \tikzstyle{di}=[diamond,thick,draw=blue!75,minimum size=4mm]

  \node[cir] (1)            {1};
  \node[cir] (2) [right =1.6cm of 1]                    {2};
  \node[cir] (3) [right  =1.6cm of 2]      {3};
  \node[cir] (4) [above =1.2cm of 3]                 {4};
  \node[cir] (5) [left =1.6cm of 4]                 {5};
  \node[cir] (6) [left =1.6cm of 5]      {6};
 \path (1) 
            edge[->] node {} (2)
            edge[->,blue, bend left] node {} (6) 
        
        (2)
            edge[->] node {} (3)
            edge[->, blue, bend left] node {} (5)
        (3)
            edge[->] node {} (4)
            edge[->, blue, bend left] (4)
        (4)
            edge[->] node {} (5)
            edge[->,blue, bend left] (3)
        (5)
            edge[->] node {} (6)
            edge[->,blue,bend left] node {} (2)
        (6)
            edge[->,blue,bend left] node {} (1);
\end{tikzpicture}}
    }
%no space
\hfill
\subfloat[Reverse stockinette, corresponding to the Eulerian edges being in the front.]{\label{fig:reverse_stockinette}
\centering

\includegraphics[width=0.45\linewidth,trim={0 15cm 0 15cm},clip]{images/purl.jpeg}
}

\subfloat[If given different orientations for the Eulerian edges, we cannot knit this object.  Here the loops must intersect instead of going around each other.]{\label{fig:not_knitting}
\centering
\resizebox{0.5\columnwidth}{!}{
\begin{tikzpicture}[->,>=stealth',shorten >=1pt,auto,node distance=2.1cm, semithick,black]
    \tikzstyle{state} = [draw=none,fill=none,right]
    \tikzstyle{rec} = \tikzstyle{transition}=[rectangle,thick,draw=blue!75,minimum size=4mm]
    \tikzstyle{cir}=[ellipse,thick,draw=black,minimum size=4mm, text=black]
    \tikzstyle{di}=[diamond,thick,draw=blue!75,minimum size=4mm]

  \node[cir] (1)            {1};
  \node[cir] (2) [right =1.6cm of 1]                    {2};
  \node[cir] (3) [right  =1.6cm of 2]      {3};
  \node[cir] (4) [above =1.2cm of 3]                 {4};
  \node[cir] (5) [left =1.6cm of 4]                 {5};
  \node[cir] (6) [left =1.6cm of 5]      {6};
 \path (1) 
            edge[->] node {} (2)
            edge[->,blue, bend left] node {} (6) 
        
        (2)
            edge[->] node {} (3)
            edge[->, blue, bend left] node {} (5)
        (3)
            edge[->] node {} (4)
            edge[->, blue, bend left] (4)
        (4)
            edge[->] node {} (5)
            edge[->,red, bend left] (3)
        (5)
            edge[->] node {} (6)
            edge[->,red,bend left] node {} (2)
        (6)
            edge[->,red,bend left] node {} (1);
\end{tikzpicture}}
    }
%no space
\hfill
% \subfloat[No knitting object corresonds to the given graph.]{\label{fig:ham_3_knit}
% \centering

% \includegraphics[width=0.45\linewidth]{images/3.png}
% }

\caption{An example of how information on the Eulerian edges can change the knitted object.}
\label{fig:stockinette_examples}
\end{figure}

\begin{figure}[p]

\centering
\subfloat[Graph view with defined Hamiltonian path in red.]{\label{fig:basic_ham}
\centering
\resizebox{0.5\columnwidth}{!}{
\begin{tikzpicture}[->,>=stealth',shorten >=1pt,auto,node distance=2.1cm, semithick,black!30!blue]
    \tikzstyle{state} = [draw=none,fill=none,right]
    \tikzstyle{rec} = \tikzstyle{transition}=[rectangle,thick,draw=blue!75,minimum size=4mm]
    \tikzstyle{cir}=[ellipse,thick,draw=black!30!blue,minimum size=4mm, text=black!30!blue]
    \tikzstyle{di}=[diamond,thick,draw=blue!75,minimum size=4mm]

  \node[cir] (1)            {1};
  \node[cir] (2) [right =1.6cm of 1]                    {2};
  \node[cir] (3) [right  =1.6cm of 2]      {3};
  \node[cir] (4) [above =1.2cm of 3]                 {4};
  \node[cir] (5) [left =1.6cm of 4]                 {5};
  \node[cir] (6) [left =1.6cm of 5]      {6};
 \path (1) 
            edge[->,red] node {} (2)
            edge[-] node {} (6) 
        
        (2)
            edge[->,red] node {} (3)
            edge[-] node {} (5)
        (3)
            edge[->,red] node {} (4)
        (4)
            edge[->,red] node {} (5)
        (5)
            edge[->,red] node {} (6);
\end{tikzpicture}}
    }
%no space
\hfill
\subfloat[Knitting object created from the graph, note some basic stockinette is put around the graph-defined area for fabric stability.]{\label{fig:ham_knit}
\centering

\includegraphics[width=0.45\linewidth]{images/1.png}
}

\subfloat[Graph view with defined Hamiltonian path in red.  Here we begin our path with node 2, which gives a different stitch pattern.]{\label{fig:ham_2}
\centering
\resizebox{0.5\columnwidth}{!}{
\begin{tikzpicture}[->,>=stealth',shorten >=1pt,auto,node distance=2.1cm, semithick,black!30!blue]
    \tikzstyle{state} = [draw=none,fill=none,right]
    \tikzstyle{rec} = \tikzstyle{transition}=[rectangle,thick,draw=blue!75,minimum size=4mm]
    \tikzstyle{cir}=[ellipse,thick,draw=black!30!blue,minimum size=4mm, text=black!30!blue]
    \tikzstyle{di}=[diamond,thick,draw=blue!75,minimum size=4mm]

  \node[cir] (1)            {2};
  \node[cir] (2) [right =1.6cm of 1]                    {3};
  \node[cir] (3) [right  =1.6cm of 2]      {4};
  \node[cir] (4) [above =1.2cm of 3]                 {5};
  \node[cir] (5) [left =1.6cm of 4]                 {6};
  \node[cir] (6) [left =1.6cm of 5]      {1};
 \path (1) 
            edge[->,red] node {} (2)
            edge[-] node {} (6) 
            edge[-] node {} (4)
        
        (2)
            edge[->,red] node {} (3)
        (3)
            edge[->,red] node {} (4)
        (4)
            edge[->,red] node {} (5)
        (5)
            edge[->,red] node {} (6);
\end{tikzpicture}}
    }
%no space
\hfill
\subfloat[Knitting object created from the graph, note some basic stockinette is put around the graph-defined area for fabric stability.]{\label{fig:ham_2_knit}
\centering

\includegraphics[width=0.45\linewidth]{images/4.png}
}

\subfloat[Graph view with defined Hamiltonian path in red.  Here we put the first four nodes on the first row, which gives a different knitted object.]{\label{fig:ham_3}
\centering
\resizebox{0.5\columnwidth}{!}{
\begin{tikzpicture}[->,>=stealth',shorten >=1pt,auto,node distance=2.1cm, semithick,black!30!blue]
    \tikzstyle{state} = [draw=none,fill=none,right]
    \tikzstyle{rec} = \tikzstyle{transition}=[rectangle,thick,draw=blue!75,minimum size=4mm]
    \tikzstyle{cir}=[ellipse,thick,draw=black!30!blue,minimum size=4mm, text=black!30!blue]
    \tikzstyle{di}=[diamond,thick,draw=blue!75,minimum size=4mm]

  \node[cir] (1)            {1};
  \node[cir] (2) [right =1.6cm of 1]                    {2};
  \node[cir] (3) [right  =1.6cm of 2]      {3};
  \node[cir] (4) [right =1.2cm of 3]                 {4};
  \node[cir] (5) [above =1.6cm of 4]                 {5};
  \node[cir] (6) [left =1.6cm of 5]      {6};
 \path (1) 
            edge[->,red] node {} (2)
            edge[-] node {} (6) 
        
        (2)
            edge[->,red] node {} (3)
            edge[-] node {} (5)
        (3)
            edge[->,red] node {} (4)
        (4)
            edge[->,red] node {} (5)
        (5)
            edge[->,red] node {} (6);
\end{tikzpicture}}
    }
%no space
\hfill
\subfloat[Knitting object created from the graph, note some basic stockinette is put around the graph-defined area for fabric stability.]{\label{fig:ham_3_knit}
\centering

\includegraphics[width=0.45\linewidth]{images/3.png}
}

\caption{An example of how different Hamiltonian paths can lead to different knitted objects.}
\label{fig:total_ham_path_fig}
\end{figure}
